# Supplementary material for: The Joneses Visit an Economics Lab
Source: arXiv:2607.07353 source file (2026-09-17)
Supplement: Supplementary file 1 [file additional_figures.tex]

\documentclass[12pt]{article}
\bibliographystyle{apalike}   % or plain, etc.

\input{preambleR}

\begin{document}

\section{Adjustments by ranks}

\begin{figure}[H]
    \centering
    \includegraphics[width=0.5\linewidth]{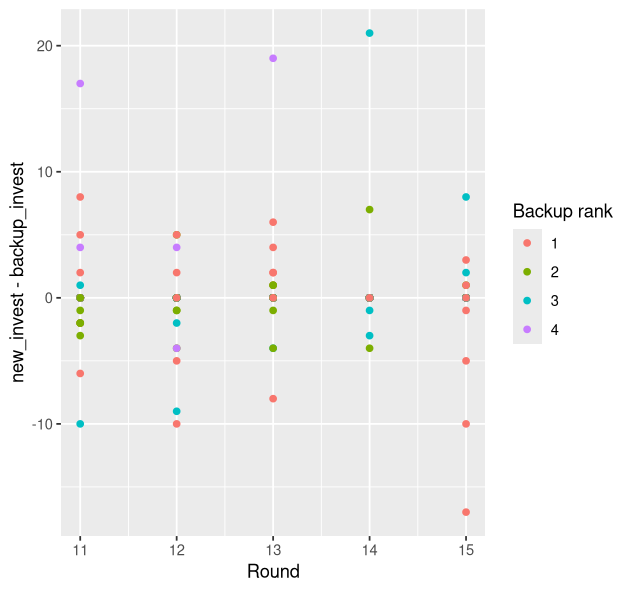}
    \caption{Backup rank $=$ rank before the adjustment is made. 
    \\
    y-axis = adjustment in investment
    \\
    x-axis = period
    }
    \label{fig:placeholder}
\end{figure}

\begin{figure}[H]
    \centering
    \includegraphics[width=0.5\linewidth]{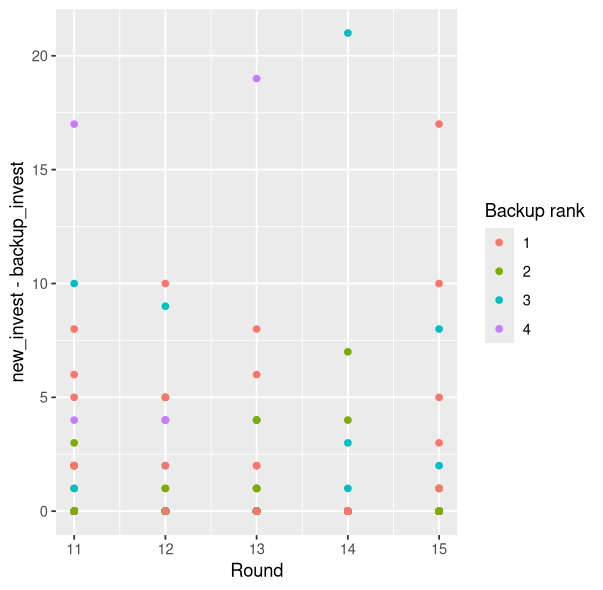}
    \caption{Backup rank $=$ rank before the adjustment is made. 
    \\
    y-axis = absolute adjustment in investment
    \\
    x-axis = period
    }
    \label{fig:placeholder}
\end{figure}

\begin{figure}[H]
    \centering
    \includegraphics[width=0.5\linewidth]{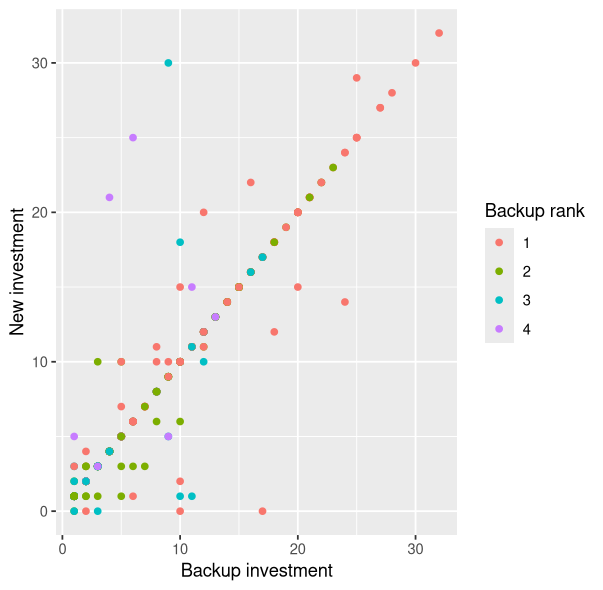}
    \caption{Scatter plot: New Invest, Backup Invest; Colors = Backup Rank
    }
    \label{fig:placeholder}
\end{figure}

\begin{figure}[H]
    \centering
    \includegraphics[width=0.5\linewidth]{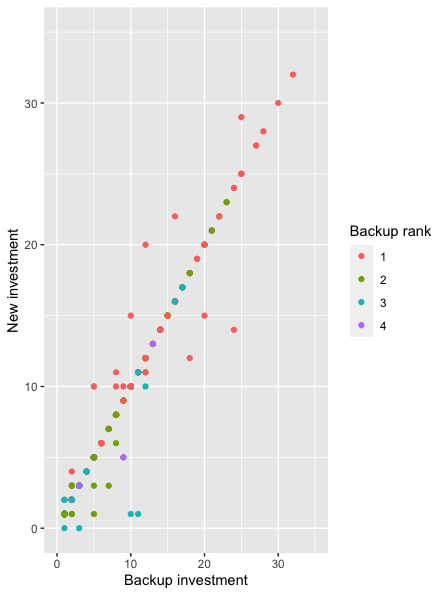}
    \caption{New vs Backup Investment while staying within the same rank}
    \label{fig:placeholder}
\end{figure}

\begin{figure}[H]
    \centering
    \includegraphics[width=0.5\linewidth]{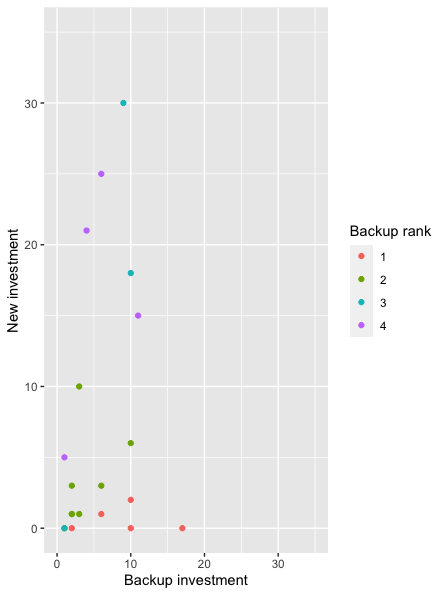}
    \caption{New vs Backup Investment while changing the rank}
    \label{fig:placeholder}
\end{figure}

\begin{figure}[H]
    \centering
    \includegraphics[width=0.5\linewidth]{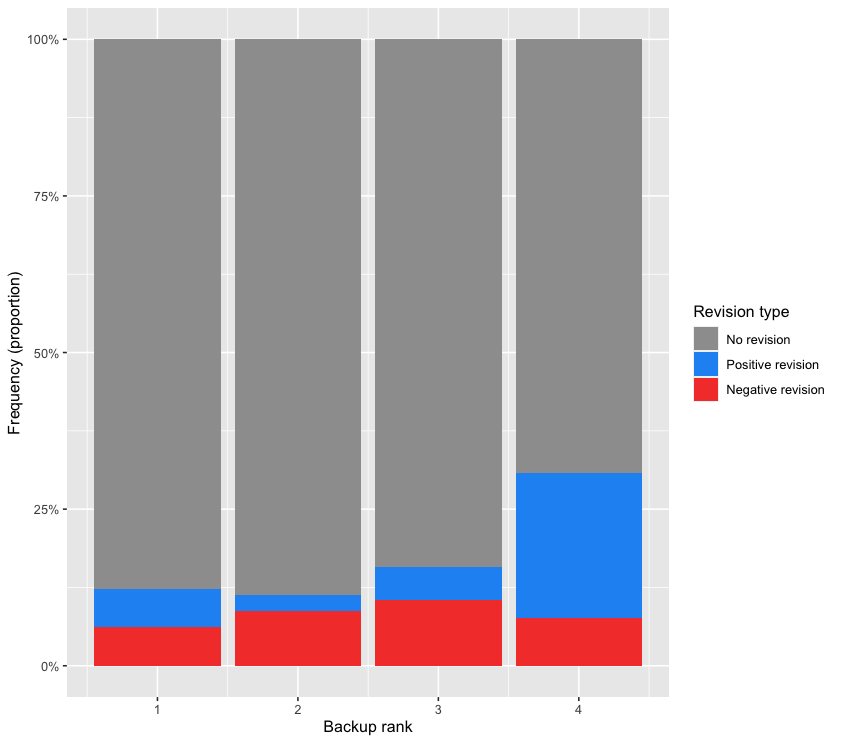}
    \caption{HIST: frequency of adjustments by rank
    \\
    (controlling for backup invest $>$ 3)}
    \label{fig:placeholder}
\end{figure}

\begin{figure}[H]
    \centering
    \includegraphics[width=0.5\linewidth]{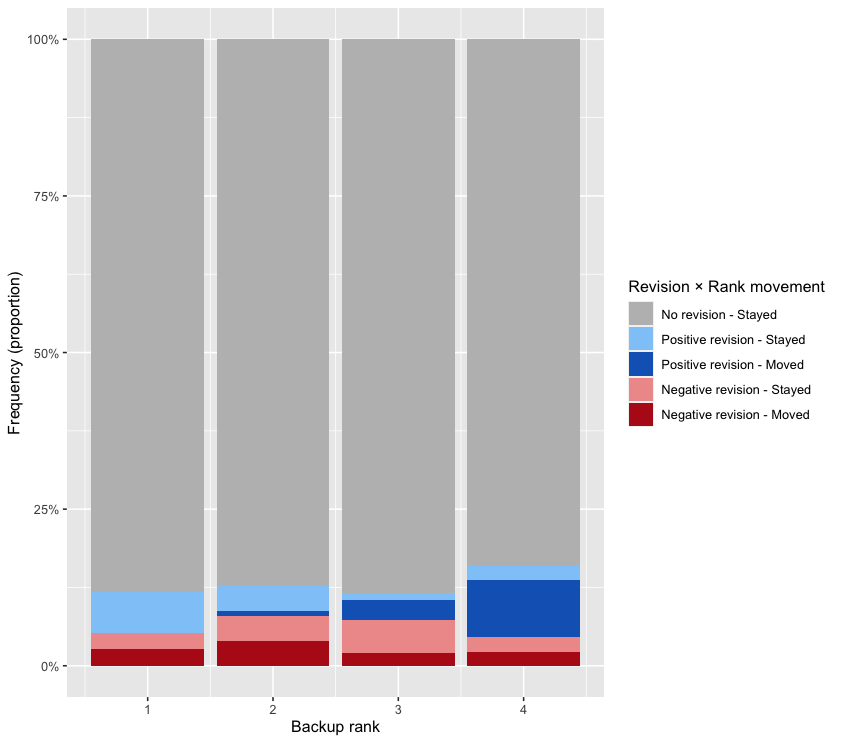}
    \caption{New vs Backup Investment while changing the rank}
    \label{fig:placeholder}
\end{figure}

\begin{table}[H]
\centering
\begin{tabular}{rrr}
  \hline
Backup Rank & Negative & Positive \\ 
  \hline
1 &   9 &  12 \\ 
  2 &  11 &   5 \\ 
  3 &   6 &   4 \\ 
  4 &   1 &   4 \\ 
   \hline
\end{tabular}
\caption{Contingency Table: Positive vs Negative Revisions by Backup Rank} 
\label{tab:revisions}
\end{table}

\section{Pride and Envy}

\begin{figure}[H]
    \centering
    \includegraphics[width=0.5\linewidth]{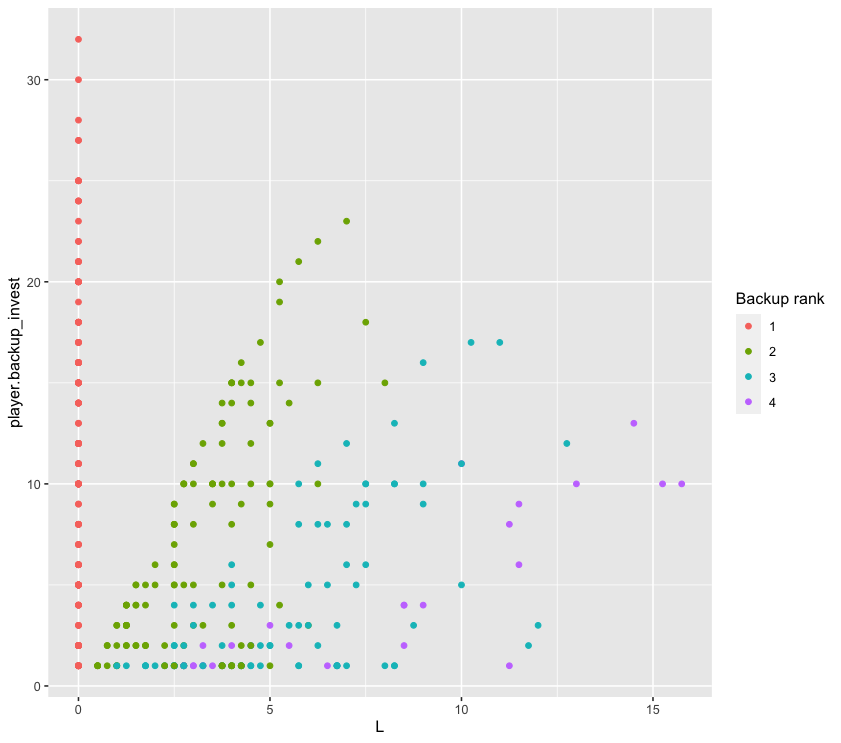}
    \caption{Backup investing by L and by Rank}
    \label{fig:placeholder}
\end{figure}

\begin{figure}[H]
    \centering
    \includegraphics[width=0.5\linewidth]{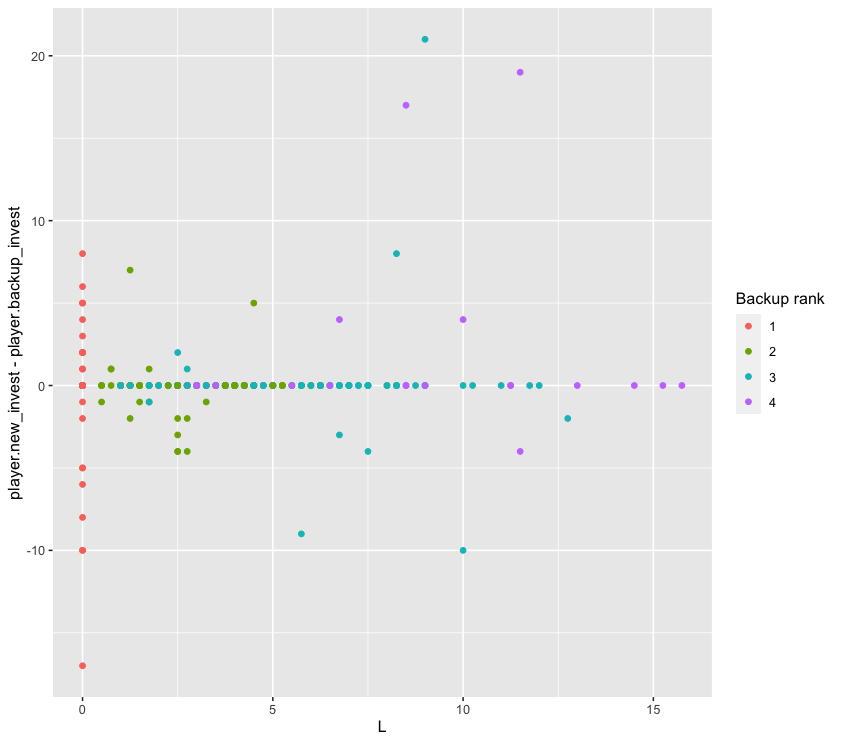}
    \caption{Diff investment by L and by Rank}
    \label{fig:placeholder}
\end{figure}

\begin{figure}[H]
    \centering
    \includegraphics[width=0.5\linewidth]{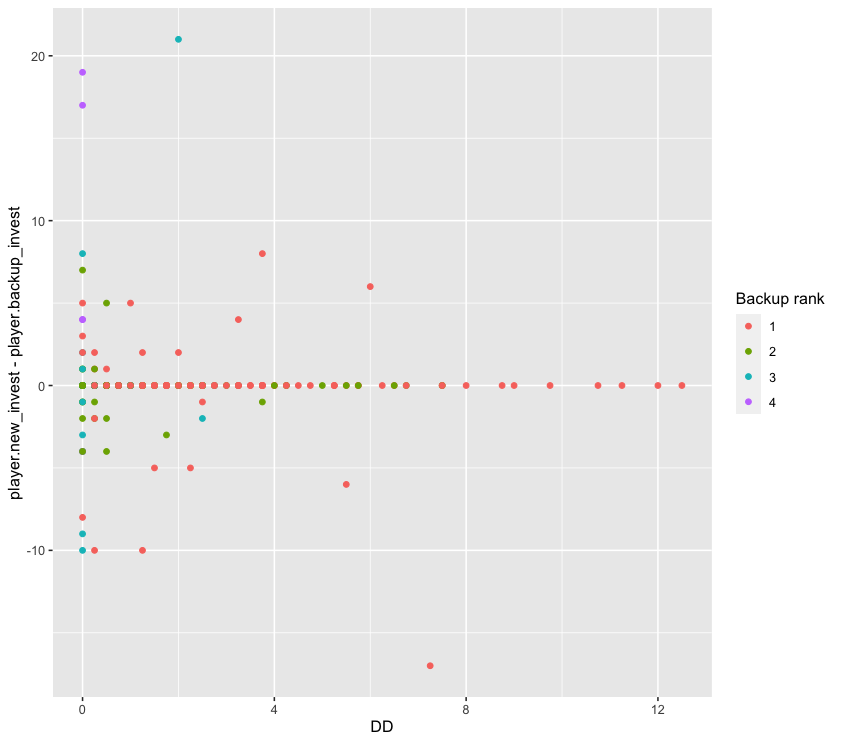}
    \caption{Diff investment by DD and by Rank}
    \label{fig:placeholder}
\end{figure}

\begin{figure}[H]
    \centering
    \includegraphics[width=0.5\linewidth]{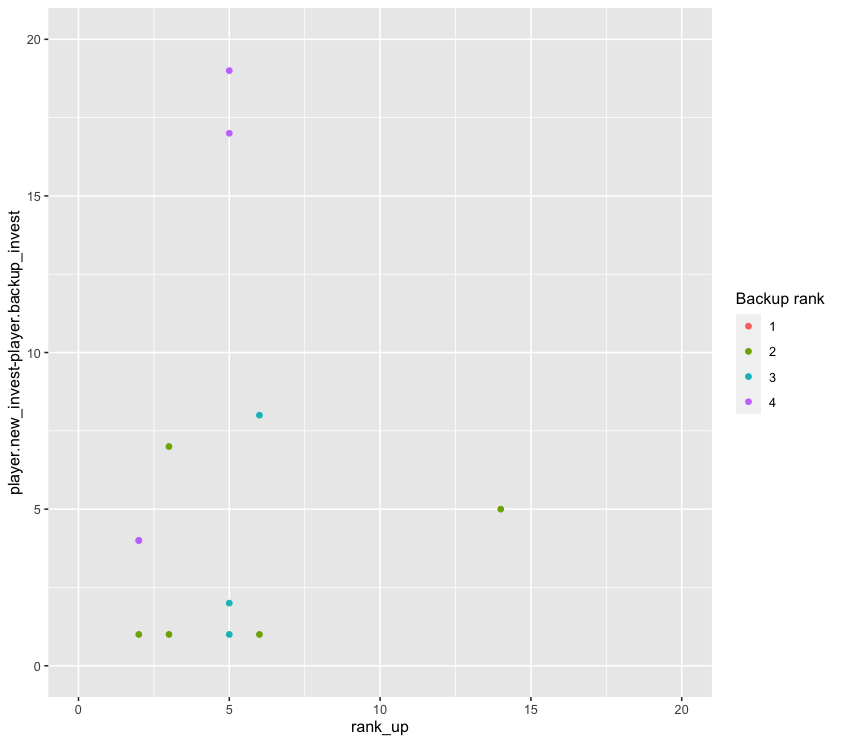}
    \caption{(positive) Diff investment vs RankUp}
    \label{fig:placeholder}
\end{figure}

\begin{figure}[H]
    \centering
    \includegraphics[width=0.5\linewidth]{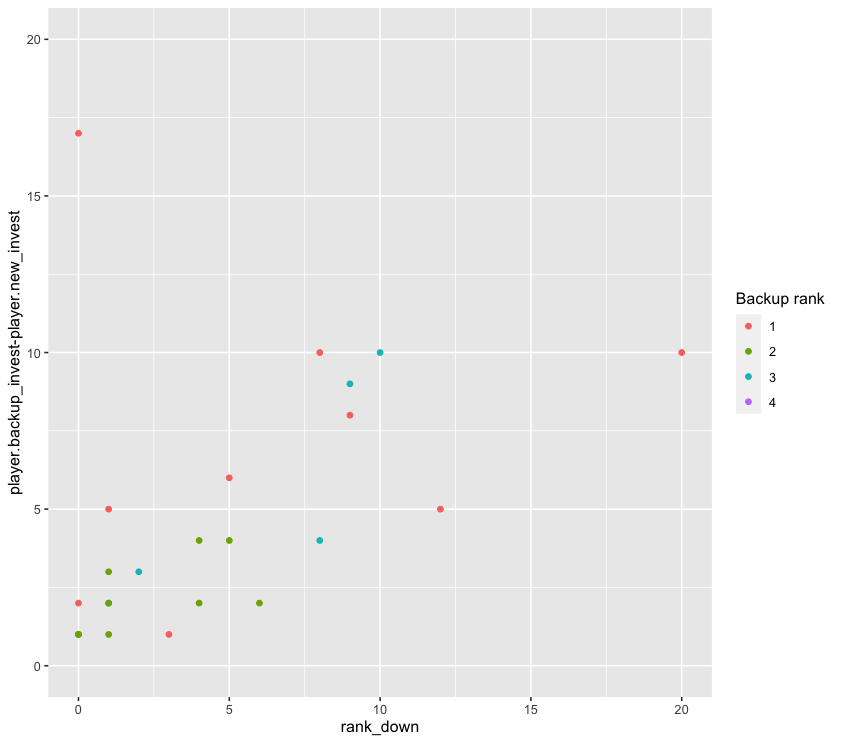}
    \caption{(negative) Diff investment vs RankDown}
    \label{fig:placeholder}
\end{figure}

\begin{figure}[H]
    \centering
    \includegraphics[width=0.5\linewidth]{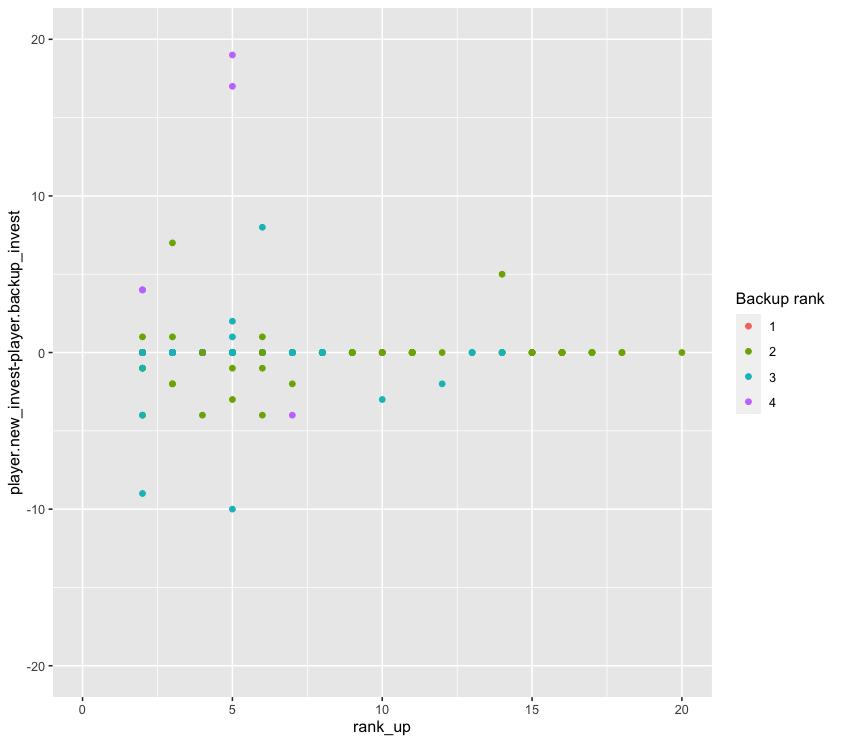}
    \caption{(all) Diff investment vs RankUP}
    \label{fig:placeholder}
\end{figure}

\begin{table}[H]
\begin{center}
\begin{tabular}{l c c c c}
\hline
 & Model 1 & Model 2 & Model 3 & Model 4 \\
\hline
peers\_backup\_mean                   & $3.04^{***}$ &                 & $2.74^{*}$ &                 \\
                                      & $(0.76)$     &                 & $(1.18)$   &                 \\
player.num\_correct                   & $-0.11$      & $-0.20^{\circ}$ & $-0.12$    & $-0.14^{\circ}$ \\
                                      & $(0.09)$     & $(0.11)$        & $(0.10)$   & $(0.08)$        \\
UD                                    &              & $1.60^{***}$    & $0.35$     & $1.16^{***}$    \\
                                      &              & $(0.32)$        & $(0.60)$   & $(0.30)$        \\
DD                                    &              &                 &            & $1.03^{**}$     \\
                                      &              &                 &            & $(0.33)$        \\
\hline
Num. obs.                             & $150$        & $150$           & $150$      & $150$           \\
\hline
\multicolumn{5}{l}{\scriptsize{$^{***}p<0.001$; $^{**}p<0.01$; $^{*}p<0.05$; $^{\circ}p<0.1$}}
\end{tabular}
\caption{
Regression specification using both mean-UD and UD-DD specifications.
\\
Subsample of active players :  backup invest $>$ 3.
\\
FEs: round number, backup  rank
\\
Clustering s.e.-s: participant-level
}
\label{table:coefficients}
\end{center}
\end{table}

\end{document}
